# Supplementary material for: Delocalized Excitation Transfer in Open Quantum Systems with Long-Range Interactions
Source: arXiv:2502.04383 source file (2025-07-03)

(a)

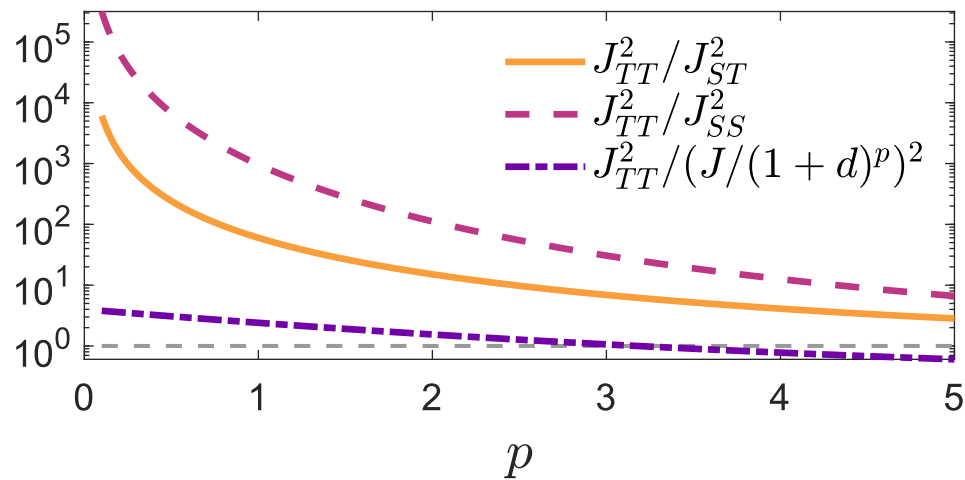

(b)

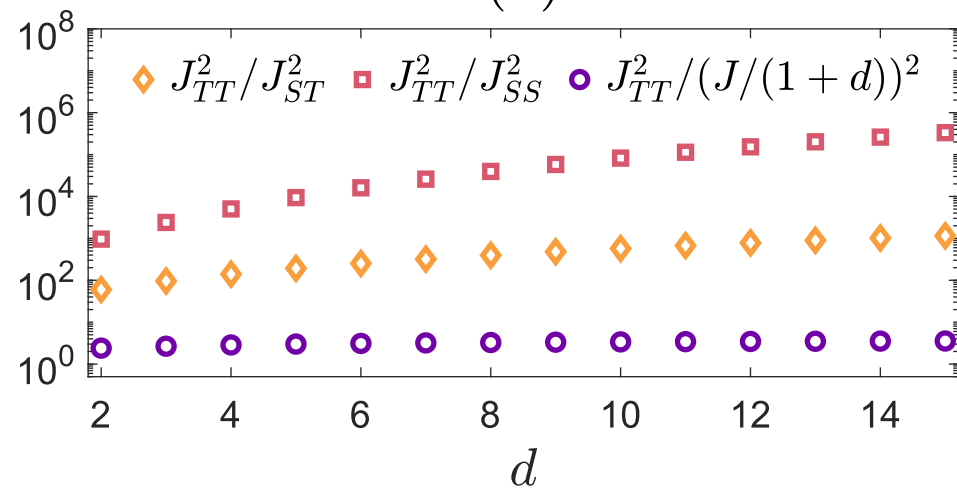

Supplement: Supplementary file 1 [file Fig1Supp.pdf]
